# Supplementary material for: Pair Correlations and Photoassociation Dynamics of Two Atoms in an Optical Tweezer
Source: arXiv:2009.00147 source file (2021-01-25)
Supplement: Supplementary file 1 [file Supplemental.pdf]

# Supplemental Material for: Pair Correlations and Photoassociation Dynamics of Two Atoms in an Optical Tweezer

Marvin Weyland,<sup>1,2</sup> Stuart S. Szigeti,<sup>3</sup> Poramaporn Ruksasakchai,<sup>1,2</sup> Rhys Hobbs,<sup>2</sup> and Mikkell F. Andersen<sup>1,2</sup>

<sup>1</sup>*The Dodd-Walls Centre for Photonic and Quantum Technologies, University of Otago, Dunedin, New Zealand*

<sup>2</sup>*Department of Physics, University of Otago, Dunedin, New Zealand*

<sup>3</sup>*Department of Quantum Science, Research School of Physics,  
The Australian National University, Canberra 2601, Australia*

## RECONSTRUCTION OF OPTICAL TWEezer'S POPULATIONS

When reconstructing the probability of finding a certain number of atoms in the tweezer after photoassociation, as shown in Fig. 2 we first record baseline photon count distributions by capturing atoms without exposure to photoassociation light. We obtain the initial atom loading state from an EMCCD image before merging the traps and sorting cases with zero-, one-, and two-atom initial loading. We perform these baseline measurements several thousand times to obtain photon count distributions for each possible number of atoms in the tweezer. These measurements contain 3.5% single atom loss from the merging process which can be identified in the photon counts of one-atom loading cases as events with close to zero photons detected. We correct the baseline photon count distributions of one-atom and two-atom loading cases for this loss and fit a combination of the resulting baseline distributions to the experimental photon count distributions, which we obtain from photoassociation measurements, as shown in Fig. S1.

Since the parameter space of the fit is restricted to two free parameters between 0% and 100% corresponding to the probability of finding zero or one atom, we can ensure that our fitting algorithm finds the global minimum of the squared residuals by probing the whole parameter space with a 5%-step size, followed by probing the area around the global minimum with a 0.25%-step size. We create 1000 bootstrap resampling data sets from this initial fit to obtain the final parameters and their standard deviations [29]. To analyze experiments with three atoms, we extend the described process to include a three-atom photon count distribution.

## FIT OF PHOTOASSOCIATION DYNAMICS

The dynamics of the photoassociation process can be described by a set of coupled rate equations. In the specific case of two atoms in an optical tweezer, we describe

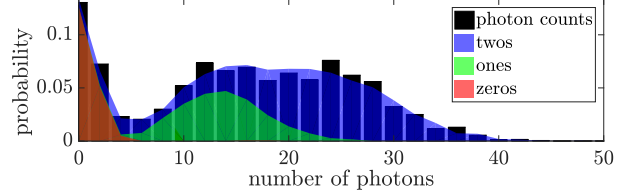

FIG. S1. Example of a photon distribution obtained from 3600 iterations of an experiment (bars) and fitted with photon distributions for zero, one and two atoms (stacked, shaded areas).

the evolution of the populations by

$$\begin{pmatrix} \dot{p}_0 \\ \dot{p}_1 \\ \dot{p}_2^n \\ \dot{p}_2^p \end{pmatrix} = \begin{pmatrix} 0 & \gamma_1 & \gamma_2^n & \gamma_2^p \\ 0 & -\gamma_1 & 2\gamma_1 & 2\gamma_1 \\ 0 & 0 & -\gamma_2^n - 2\gamma_1 & 0 \\ 0 & 0 & 0 & -\gamma_2^p - 2\gamma_1 \end{pmatrix} \begin{pmatrix} p_0 \\ p_1 \\ p_2^n \\ p_2^p \end{pmatrix}, \quad (\text{S1})$$

where  $p_i(t)$  is the probability of finding  $i$  atoms in the tweezer after we expose it to photoassociation light for a specific time  $t$ . Single-atom loss occurs with a rate  $\gamma_1$  due to collisions of the atoms with background gas in the vacuum chamber on timescales much longer than photoassociation. The two different probabilities for the two-atom population describe the tweezer states whose relative-motional wavefunctions have a peak ( $p_2^p$ ) or a node ( $p_2^n$ ) at zero separation. Our measured probability for the total two-atom population is thus  $p_2 = p_2^n + p_2^p$ . In our analysis we compare this two-timescale model with the one-timescale model for which the second two-atom population is removed. When analyzing the evolution of a three-atom system, the equation is extended to include a probability for three-atom population but no three-atom loss. In this extension of the equation, single atom loss starting from a three-atom population is assumed to populate both two-atom populations ( $p_2^n$  and  $p_2^p$ ) equally. conditions.

## TWO-TIMESCALE DYNAMICS WITH DIFFERENT PHOTOASSOCIATION PARAMETERS

Most measurements were performed at a peak laser intensity of  $580 \text{ W cm}^{-2}$ . Some additional measurement

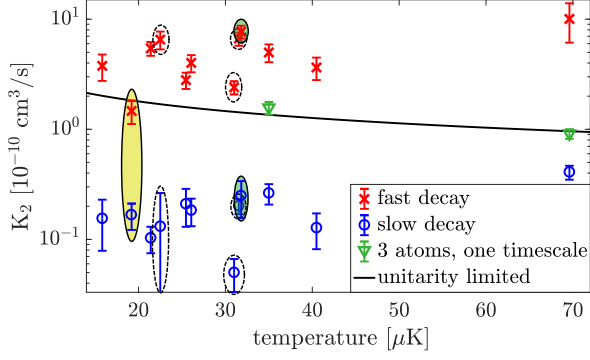

FIG. S2. Photoassociation rate coefficients for pair-correlated two-atom wavefunctions (fast decay, red crosses) and pair-anticorrelated two-atom wavefunctions (slow decay, blue circles) compared to the many-atom unitarity-limited rate coefficient. Specially marked measurements are described in the text.

were performed with different parameters and are shown in Fig. S2. The points in dashed circles were taken at a peak intensity of  $230 \text{ W cm}^{-2}$ , closer to the intensity which showed the highest rate coefficient. The solid-encircled points were taken without chopping the tweezer and with a photoassociation light intensity of  $580 \text{ W cm}^{-2}$  (yellow filled) and  $21 \text{ W cm}^{-2}$  (green filled). These results rule out our experimental procedure of chopping tweezer and photoassociation light as a possible source of the observed two-timescale dynamics. However, the measured rate coefficients at continuous trapping and photoassociation light shows that the maximum rate coefficient is reached at a lower photoassociation light intensity of around  $21 \text{ W cm}^{-2}$  and the rate coefficient is lower at  $580 \text{ W cm}^{-2}$ , as expected for intensities above the saturation intensity. This difference might arise from the chopping of the photoassociation light. The peak intensity during the chopping operation is not reached for the whole on-time of the photoassociation laser.

We measured the pulse shape using a fast photo-diode (HFD3180-203, 80 ps rise/fall time) and a 500 MHz oscilloscope. The observed pulse shape is shown in Fig. S3. In addition to the 150 ns pulse used in our measurements we also plot a 250 ns pulse which shows that the maximum intensity is reached in the experiment. However, we observe significant rise and fall times. The maximum intensity is maintained for only 50 ns and above 50% intensity for 140 ns. The effective intensity during the on-time in chopped operation is lower than the peak power. This might in part explain the higher apparent saturation intensity in chopped operation compared to continuous photoassociation light.

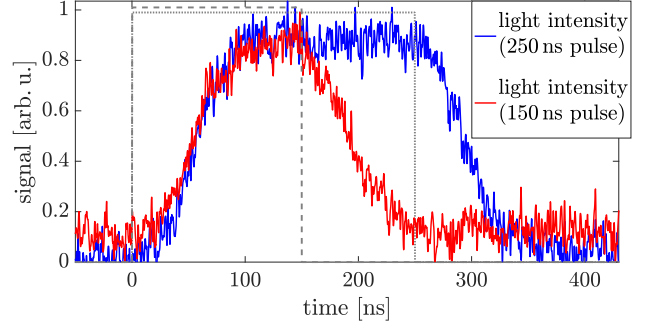

FIG. S3. Shape of the actual photoassociation pulses (150 ns) and of a longer photoassociation pulse (250 ns) for comparison. The dashed and dotted lines show the pulse shapes for triggering the 150 ns and 250 ns photoassociation pulses. They have been shifted in time by a common value to have their falling edge coincide with the beginning of the fall time of the photoassociation pulses.

## STATISTICAL ANALYSIS OF FITS

We assess the validity of our two-timescale model when fitting it to measurements from 18 different experimental runs using different atom temperatures and photoassociation powers as well as changing the preparation of the atoms from the  $|F = 2, m = 0\rangle$  state to a mix of all five  $m$ -states. A  $\chi^2$ -test [23] rejects the one-timescale model for 17 of those measurements at the 5% level of significance, whereas the two-timescale model is rejected for only 4 measurements. Using the two-timescale model improves the reduced  $\chi^2$ -values by a factor of 7 compared to the one-timescale model. Even in the 4 data sets for which the two-timescale model was rejected, it still resulted in an improvement by a factor of 3.

## CALCULATION OF RATE COEFFICIENT

Eq. (6) shows the relation between the pair-loss rate  $\gamma_2$  in the experiment and the underlying rate coefficient  $K_2$ . It requires knowledge of the thermal density of atoms in the optical tweezer, which is given by [28]

$$n(\mathbf{r}) = n_0 \exp\left(\frac{-(U(\mathbf{r}) - U_0)}{k_B T}\right), \quad (\text{S2})$$

where  $n_0$  is the peak density. At the temperatures used in our experiments, the atoms are in low trap states. Therefore, the Gaussian trap can be approximated as the harmonic potential

$$n(\mathbf{r}) = n_0 \exp\left(\frac{-m\omega_r^2 r^2}{2k_B T}\right) \exp\left(\frac{-m\omega_z^2 z^2}{2k_B T}\right). \quad (\text{S3})$$

We measured the radial frequency  $\omega_r$  using Raman side-band spectroscopy and obtained the axial frequency  $\omega_z$

from the previously measured ratio between radial and axial frequencies in our tweezer [22].

### DETERMINATION OF SATURATION INTENSITY

The expected saturation intensity can be found from the resonance width as a function of photoassociation intensity [25, 26]. We measured the width of the photoassociation resonance in an intensity range from  $12 \text{ W cm}^{-2}$  (0.1 mW beam power) to  $2300 \text{ W cm}^{-2}$  (200 mW beam power) and used a weighted linear fit to obtain a linewidth of  $(12 \pm 6) \text{ MHz}$  at zero intensity, which serves as an upper bound for the natural linewidth. We find the saturation intensity - where the observed linewidth is twice the natural linewidth - to be  $(200 \pm 100) \text{ W cm}^{-2}$ . While this method gives large errors, it does not rely on any rate measurement and the expected saturation intensity is in the range where we performed our experiments.

### DETAILS OF NUMERICAL SIMULATION

We numerically solve Eq. (3) by expanding  $\psi(\mathbf{r})$  on a finite basis of even-parity eigenstates of  $H_{\text{rel}}(\mathbf{r})$ :  $\psi(\mathbf{r}, t) = \sum_{\mathbf{n} \leq E_{\text{cut}}} c_{\mathbf{n}}(t) \phi_{\mathbf{n}}(\mathbf{r})$ , where  $\mathbf{n} = (n_x, n_y, n_z)$  and the sum is over all even-parity eigenstates with energy  $\varepsilon_{\mathbf{n}} = \sum_{i=x,y,z} \hbar \omega_i (n_i + \frac{1}{2})$  less than some energy cutoff  $E_{\text{cut}}$ . We assume our initial condition is a thermal distribu-

tion of even eigenstates of  $H_{\text{rel}}(\mathbf{r})$ . That is, in any given experiment  $\psi(\mathbf{r}, 0) = \phi_{\mathbf{n}_0}(\mathbf{r})$  with Boltzmann probability  $\mathcal{P}_{\mathbf{n}_0} = \exp(-\beta \varepsilon_{\mathbf{n}_0}) / \mathcal{Z}$ , where  $\beta = 1/k_{\text{B}}T$  and the partition function  $\mathcal{Z}$  has an analytic expression (see for example Supplementary Note 5 of [16]):

$$\mathcal{Z} = \mathcal{Z}_x^{\text{even}} \mathcal{Z}_y^{\text{even}} \mathcal{Z}_z^{\text{even}} + \mathcal{Z}_x^{\text{odd}} \mathcal{Z}_y^{\text{odd}} \mathcal{Z}_z^{\text{even}} + \mathcal{Z}_x^{\text{odd}} \mathcal{Z}_y^{\text{even}} \mathcal{Z}_z^{\text{odd}} + \mathcal{Z}_x^{\text{even}} \mathcal{Z}_y^{\text{odd}} \mathcal{Z}_z^{\text{odd}}, \quad (\text{S4})$$

where

$$\mathcal{Z}_i^{\text{even}} = \sum_{m_i=0}^{\infty} e^{-\beta \hbar \omega_i (2m_i + 1/2)} = \frac{e^{-\beta \hbar \omega_i / 2}}{1 - e^{-2\beta \hbar \omega_i / 2}}, \quad (\text{S5})$$

$$\mathcal{Z}_i^{\text{odd}} = \sum_{m_i=0}^{\infty} e^{-\beta \hbar \omega_i [(2m_i + 1) + 1/2]} = \frac{e^{-3\beta \hbar \omega_i / 2}}{1 - e^{-2\beta \hbar \omega_i / 2}}. \quad (\text{S6})$$

We choose  $E_{\text{cut}}$  such that both  $\sum_{\varepsilon_{\mathbf{n}} \leq E_{\text{cut}}} \mathcal{P}_{\mathbf{n}} \gtrsim 0.996$  and coupling to the highest-energy, sparsely-occupied modes is negligible. For the computational resources at our disposal, these conditions limit our calculations to temperatures no greater than  $10.5 \mu\text{K}$  - roughly half the lowest temperature investigated experimentally.

In this basis, evolution under Eq. (3) corresponds to

$$i\hbar \dot{c}_{\mathbf{n}} = \varepsilon_{\mathbf{n}} c_{\mathbf{n}} - i \sum_{\mathbf{m} \leq E_{\text{cut}}} V_{\mathbf{n}\mathbf{m}} c_{\mathbf{m}}, \quad (\text{S7})$$

where

$$V_{\mathbf{n}\mathbf{m}} = \int d\mathbf{r} \phi_{\mathbf{m}}^*(\mathbf{r}) V(\mathbf{r}) \phi_{\mathbf{n}}(\mathbf{r})$$

$$= \hbar \gamma \int_{-r_c}^{r_c} dx \phi_{m_x}^*(x) \varphi_{n_x}(x) \int_{-\sqrt{r_c^2 - x^2}}^{\sqrt{r_c^2 - x^2}} dy \phi_{m_y}^*(y) \varphi_{n_y}(y) \int_{-\sqrt{r_c^2 - x^2 - y^2}}^{\sqrt{r_c^2 - x^2 - y^2}} dz \phi_{m_z}^*(z) \varphi_{n_z}(z). \quad (\text{S8})$$

These matrix elements were numerically computed using adaptive Hermite-Legendre quadrature methods in Mathematica. Thus, for a given initial condition  $\psi(\mathbf{r}, 0) = \phi_{\mathbf{n}_0}(\mathbf{r})$ , solving Eq. (S7) allows us to compute the probability  $N_{\mathbf{n}_0}(t) = \sum_{\varepsilon_{\mathbf{n}} \leq E_{\text{cut}}} |c_{\mathbf{n}}(t)|^2$ . The total population assuming a thermal initial state is given by an incoherent sum over  $N_{\mathbf{n}_0}(t)$  weighted by the Boltzmann probability  $\mathcal{P}_{\mathbf{n}_0}$ :

$$P(t) = \sum_{\varepsilon_{\mathbf{n}_0} \leq E_{\text{cut}}} \mathcal{P}_{\mathbf{n}_0} N_{\mathbf{n}_0}(t). \quad (\text{S9})$$

This procedure was used to generate the simulation data plotted in Fig. 3.

We obtained a significant computational efficiency by

exploiting the structure of the hard-sphere potential matrix elements. Explicitly, the 1D integrals in Eq. (S8) are only non-zero if  $n_i$  and  $m_i$  are both even or both odd for  $i = x, y, z$ . Consequently, Eq. (S7) can be reduced to evolution within four decoupled subspaces, corresponding to basis states spanned by even-parity eigenstates  $\phi_{\mathbf{n}}(\mathbf{r})$  where (eee)  $n_x, n_y, n_z$  are all even, (eoo)  $n_x$  is even and  $n_y, n_z$  are odd, (oeo)  $n_x, n_z$  odd and  $n_y$  even, and (ooo)  $n_x, n_y$  odd and  $n_z$  even. Physically, only states in the ‘eee’ subspace have a non-zero density at relative co-ordinate  $\mathbf{r} = 0$ . It is therefore states in this subspace that decay the fastest under our photoassociation model and which are predominantly responsible for the fast timescale decay shown in Fig. 2.
